# Supplementary material for: Quantum Dot-Based Parametric Amplifiers
Source: arXiv:2111.11825 source file (2021-12-02)
Supplement: Supplementary file 1 [file supplementary.pdf]

# Supplementary Material: Quantum Dot-Based Parametric Amplifiers


Laurence Cochrane,[1,2,*] Theodor Lundberg,[3,4] David J. Ibberson,[2] Lisa Ibberson,[4] Louis Hutin,[5] Benoit Bertrand,[5] Maud Vinet,[5] Nadia Stelmashenko,[6] Jason W. A. Robinson,[6] Ashwin A. Seshia,[1] and M. Fernando Gonzalez-Zalba[2]

[1]*Nanoscience Centre, Department of Engineering, University of Cambridge, Cambridge CB3 0FF, UK*

[2]*Quantum Motion Technologies, Windsor House, Cornwall Road, Harrogate HG1 2PW, UK*

[3]*Cavendish Laboratory, University of Cambridge, J.J. Thomson Avenue, Cambridge CB3 0HE, UK*

[4]*Hitachi Cambridge Laboratory, J.J. Thomson Avenue, Cambridge CB3 0HE, UK*

[5]*CEA/LETI-MINATEC, CEA-Grenoble, 38000 Grenoble, France*

[6]*Department of Materials Science and Metallurgy, University of Cambridge, 27 Charles Babbage Road, Cambridge CB3 0FS, United Kingdom*



(Dated: December 2, 2021)

## S1. CHARACTERISATION OF THE MICROWAVE CAVITY

Extraction of reliable values for the resonator internal and external quality factors $Q_i$ and $Q_e$ is hindered by the complication of RF calibration at millikelvin temperatures [1] and the asymmetric resonances arising from impedance mismatches in the reflectometry setup [2, 3]. To compensate for the uncalibrated standing-wave background of reflectometry readout chain, we measure the resonator response at magnetic fields up to 0.9 T (Fig. 1(a)) and use the resulting shift in frequency to infer the background amplitude transfer function (Fig. 1(b)). We account for any asymmetry by fitting a complex external Q-factor $\tilde{Q}_e$ to the background-subtracted data (Fig. 1(c)) and applying a diameter correction method [2], with the resonator reflection coefficient modelled by [4, 5]:

$$\Gamma(f) = A\left(1 - \frac{2Q_L/|\tilde{Q}_e|e^{j\phi}}{1 + 2jQ_L(f - f_0)/f_0}\right) \tag{1}$$

The extracted parameters at $B = 0\,\mathrm{T}$ are $f_0 = 1811.0\,\mathrm{MHz}$, $\beta = 1.10$, $\tilde{Q}_e = 276e^{0.33j}$ giving $Q_e = 292$, $Q_i = 323$, $Q_L = 153$, and hence a loaded bandwidth of $11.8\,\mathrm{MHz}$. Figure 1(d) shows the resonator quality factor does not degrade at high magnetic fields. As the maximum quantum capacitance of a dot-reservoir transition can be independent of magnetic field [6], this suggests any resulting quantum dot parametric amplifier would also prove resilient.

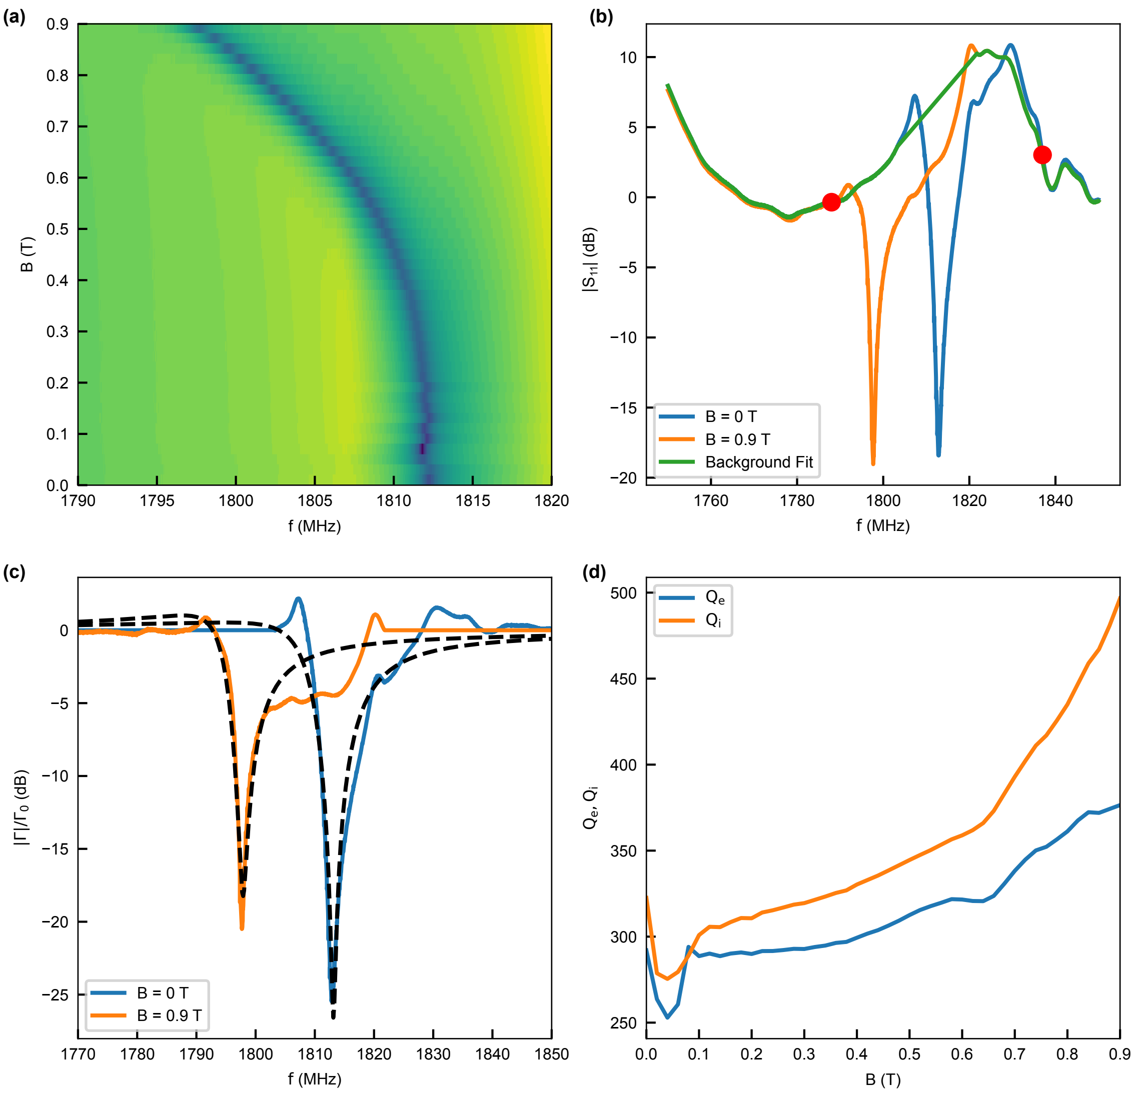


FIG. 1. Resonator parameter extraction. (a) Magnetospectroscopy of the reflection coefficient $S_1 1$ showing the variation of resonant frequency with magnetic field $B$. (b) Resonator reflection coefficient $\Gamma$ at fields $B = 0$T and 0.9 T and estimated background signal. Red points delimit the frequencies above and below which the 0 T and 0.9 T spectra overlap; this defines the width of the resonance used for background subtraction. (c) Background-subtracted response and complex external Q factor fit. (d) Variation of extracted internal and external Q-factors with magnetic field.

In the extraction of the Sisyphus resistance from the charge transition frequency shift data (Fig. 2(b) in the main text), we use a "bootstrap" method to isolate the uncalibrated standing wave background. We assume that only the internal quality factor and resonant frequency change as a function of detuning, while the excitation amplitude, external quality factor and standing wave background remain constant. Fitting the spectrum at each detuning (vertical traces in Fig. 2(b) of the main text) with a resonance response of the form of eq. (1) (constraining $\tilde{Q}_e$ and $A$ to be constant for the entire dataset), we obtain estimates for the standing wave background transfer function from the residuals of each fit. Figure 2(a) below shows example resonance fits at two detuning values $\varepsilon_1$ and $\varepsilon_2$. These residual traces show good consistency across all detunings, allowing an estimate of the background to obtained from their average. Subtracting this background from the raw data gives a corrected dataset, and allows a second set of quality factors and frequencies to be fitted with lower residual errors (fig. 2(b)).

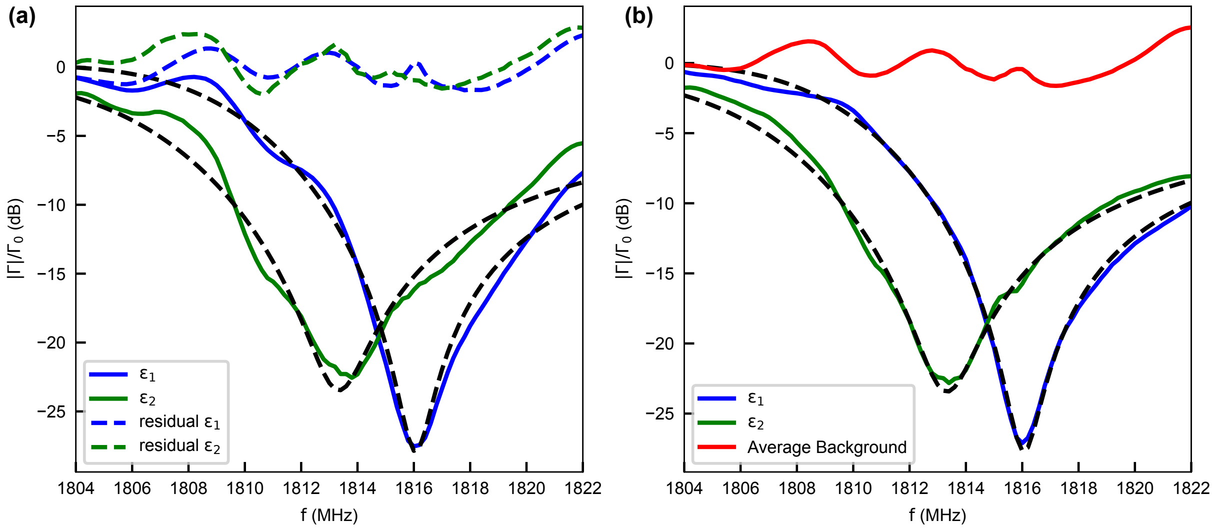


FIG. 2. (a) Reflection coefficient fits (black dashed lines) of raw reflectometry data at two different detunings and associated residuals. (b) Background-subtracted data (green and blue lines) with resonance fits (black dashed lines) and average background (red solid line).

## SEMI-CLASSICAL ANALYSIS OF THE QD PARAMETRIC AMPLIFIER

By employing a parallel small-signal equivalent circuit of the quantum dot device incorporating the quantum capacitance and Sisyphus resistance [7], we are able to analyse the performance of the QD-cavity hybrid device using a classical circuit model (Fig 3(a); Fig 1(c) in main text). The oscillatory input signal $v_f$ and pump modulation $C_Q$ are represented by:

$$\begin{aligned} v_F &= \tilde{f} + \tilde{f}^* = V_f e^{j\omega_s t} + V_f^* e^{-j\omega_s t} \\ C_Q(t) &= \tilde{p} + \tilde{p}^* = P e^{j\omega_p t} + P^* e^{-j\omega_p t} \end{aligned} \tag{2}$$

Mixing due to the non-linear quantum capacitance will produce a frequency component at $\omega_i = \omega_p - \omega_s$ (the idler mode), present in the resonator voltage $v_R$ and in the scattered wave (output) $v_B$:

$$\begin{aligned} v_R &= \tilde{v}_{rs} + \tilde{v}_{rs}^* + \tilde{v}_{ri} + \tilde{v}_{ri}^* = V_{rs} e^{j\omega_s t} + V_{rs}^* e^{-j\omega_s t} + V_{ri} e^{j\omega_i t} + V_{ri}^* e^{-j\omega_i t} \\ v_B &= \tilde{v}_{bs} + \tilde{v}_{bs}^* + \tilde{v}_{bi} + \tilde{v}_{bi}^* = V_{bs} e^{j\omega_s t} + V_{bs}^* e^{-j\omega_s t} + V_{bi} e^{j\omega_i t} + V_{bi}^* e^{-j\omega_i t} \end{aligned} \tag{3}$$

Proceeding with the circuit theory of inductive coupling gives

$$\begin{aligned} v_F + v_B &= L_2 \frac{d}{dt}(i_F - i_B) + M \frac{d}{dt} i_1 \\ v_R &= L_1 \frac{d}{dt} i_1 + M \frac{d}{dt}(i_F - i_B), \end{aligned} \tag{4}$$

while the current through the modulated quantum capacitance is given by

$$i_Q = \frac{d}{dt}(C_Q(t) v_R(t)) = \frac{d}{dt}\left[(\tilde{p} + \tilde{p}^*)(\tilde{v}_{rs} + \tilde{v}_{rs}^* + \tilde{v}_{ri} + \tilde{v}_{ri}^*)\right]. \tag{5}$$

Outside the bandwidth of the resonator, the impedance loading by the varactor is low, short-circuiting the current components of $i_Q$ and eliminating the voltage components in $v_R$. For $\omega_s \approx 2\pi f_0 \approx \omega_p/2$, the remaining terms within the resonator bandwidth at $\omega_s$ and $-\omega_i$ are given by $i_Q = j\omega_s \tilde{p} \tilde{v}_{ri}^* - j\omega_i \tilde{p}^* \tilde{v}_{rs}$. Noting that $v_F = i_F/Z_0$ and accounting for the current drawn by $C$, $R$ and the technical noise sources, equations 4 may be re-written as:

$$\begin{aligned} v_F + v_B &= \frac{L_2}{Z_0} \frac{d}{dt}(v_F - v_B) + M \frac{d}{dt}\left(\frac{v_R}{R} + C\frac{dv_R}{dt} + i_Q + i_N\right) \\ v_R &= L_1 \frac{d}{dt}\left(\frac{v_R}{R} + C\frac{dv_R}{dt} + i_Q + i_N\right) + \frac{M}{Z_0}\frac{d}{dt}(v_F - v_B) \end{aligned} \tag{6}$$

Separating the components at $\omega_s$ and $-\omega_i$ for each of the two equations and eliminating the common factors $e^{j\omega_s t}$ and $e^{-j\omega_i t}$, this can be summarised in a rank-4 matrix equation of the

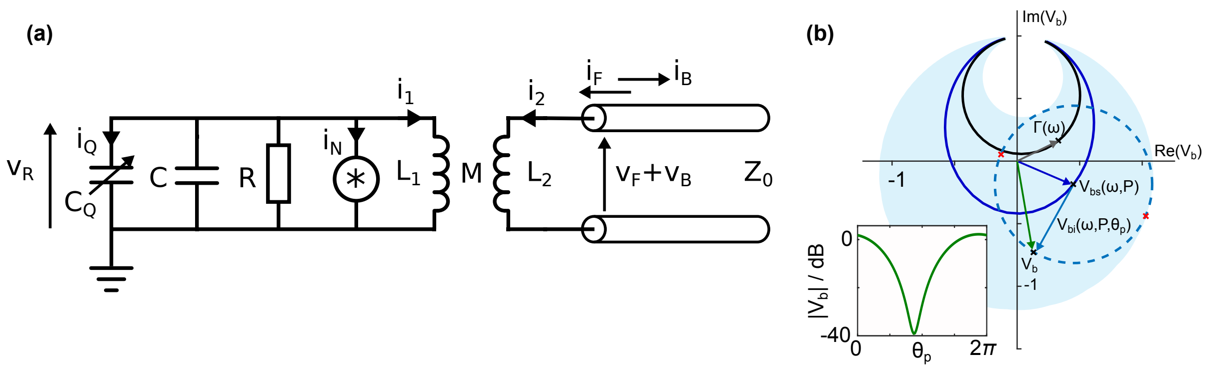


FIG. 3. (a) Small signal equivalent circuit of the QDPA. (b) Origin of degenerate phase-dependent gain, illustrated by complex (I/Q) plane loci of signal and idler mode amplitudes.

form $\mathbf{A}\mathbf{V}_{r,b} = \mathbf{B}V_f + \mathbf{Z_n}\mathbf{I_n}$:

$$\begin{bmatrix} \frac{j\omega_s M}{R} - \omega_s^2 CM & -\omega_s^2 PM & 1+\frac{j\omega_s L_2}{Z_0} & 0 \\ -\omega_i^2 P^* M & \frac{-j\omega_i M}{R} - \omega_i^2 CM & 0 & 1-\frac{j\omega_i L_2}{Z_0} \\ 1+\frac{j\omega_s L_1}{R} - \omega_s^2 CL_1 & -\omega_s^2 PL_1 & \frac{j\omega_s M}{Z_0} & 0 \\ -\omega_i^2 P^* L_1 & 1-\frac{j\omega_i L_1}{R} - \omega_i^2 CL_1 & 0 & \frac{-j\omega_i M}{Z_0} \end{bmatrix} \begin{bmatrix} V_{rs} \\ V_{ri}^* \\ V_{bs} \\ V_{bi}^* \end{bmatrix}$$
$$= \begin{bmatrix} \frac{j\omega_s L_2}{Z_0} - 1 \\ 0 \\ \frac{j\omega_s M}{Z_0} \\ 0 \end{bmatrix} V_f + \begin{bmatrix} j\omega_s M & 0 \\ 0 & j\omega_i M \\ j\omega_s L_1 & 0 \\ 0 & j\omega_i L_1 \end{bmatrix} \begin{bmatrix} I_n(\omega_s) \\ I_n^*(\omega_i) \end{bmatrix} \quad (7)$$

Figure 3(b) illustrates mechanism resulting in phase-sensitive gain by interference between the signal and idler mode phasors. The locus of signal mode $V_{bs}(\omega)$ is a transformation of the static reflection coefficient $\Gamma(\omega)$ and independent of the pump phase. The idler mode magnitude depends on frequency, while the phase $\theta_i$ tracks that of the pump signal, $\theta_p$, resulting in periodic variation in total output magnitude $V_{bs} + V_{bi}$ (see inset). The shaded area indicates the range of complex gains achievable for a given pump power by varying the frequency and pump phase.

* olc22@cam.ac.uk

[1] L. Ranzani, L. Spietz, Z. Popovic, and J. Aumentado, Two-port microwave calibration at millikelvin temperatures, Review of Scientific Instruments **84**, 034704 (2013).

[2] M. S. Khalil, M. J. A. Stoutimore, F. C. Wellstood, and K. D. Osborn, An analysis method for asymmetric resonator transmission applied to superconducting devices, Journal of Applied Physics **111**, 054510 (2012).

[3] H. Wang, S. Singh, C. R. H. McRae, J. C. Bardin, S.-X. Lin, N. Messaoudi, A. R. Castelli, Y. J. Rosen, E. T. Holland, D. P. Pappas, and J. Y. Mutus, Cryogenic single-port calibration for superconducting microwave resonator measurements, arXiv:2103.01491 [quant-ph] (2021), arXiv:2103.01491 [quant-ph].

[4] M. Kudra, J. Biznárová, A. Fadavi Roudsari, J. J. Burnett, D. Niepce, S. Gasparinetti, B. Wickman, and P. Delsing, High quality three-dimensional aluminum microwave cavities, Applied Physics Letters **117**, 070601 (2020).

[5] D. J. Ibberson, T. Lundberg, J. A. Haigh, L. Hutin, B. Bertrand, S. Barraud, C.-M. Lee, N. A. Stelmashenko, G. A. Oakes, L. Cochrane, J. W. Robinson, M. Vinet, M. F. Gonzalez-Zalba, and L. A. Ibberson, Large Dispersive Interaction between a CMOS Double Quantum Dot and Microwave Photons, PRX Quantum **2**, 020315 (2021).

[6] I. Ahmed, A. Chatterjee, S. Barraud, J. J. L. Morton, J. A. Haigh, and M. F. Gonzalez-Zalba, Primary thermometry of a single reservoir using cyclic electron tunneling to a quantum dot, Communications Physics **1**, 1 (2018).

[7] M. Esterli, R. M. Otxoa, and M. F. Gonzalez-Zalba, Small-signal equivalent circuit for double quantum dots at low-frequencies, Applied Physics Letters **114**, 253505 (2019).
